# Supplementary material for: Video Instance Matting
Source: arXiv:2311.04212 source file (2023-11-08)
Supplement: Supplementary file 1 [file ablation_fusion.tex]

\begin{table}[tb]
\centering
\resizebox{0.5\textwidth}{!}{
\begin{tabular}{c|llll}
 &  RQ$\uparrow$ & TQ$\uparrow$ & MQ$_{\mathrm{mse}}$$\uparrow$ & VIMQ$_{\mathrm{mse}}$$\uparrow$ \\ \hline
w/ Temporal Fusion  &71.59 &93.59 &54.27 &36.37   \\
w/o Temporal Fusion  &\textbf{72.72} &\textbf{93.17} &\textbf{56.52} &\textbf{38.29}  \\ \hline
\end{tabular}}
\caption{Comparisons on the Temporal Fusion. The temporal feature guidance module without temporal fusion performs better and is used in Section~\ref{ssec:temporal_guidance}. }
\vspace{-3mm}
\label{ablation_fusion}
\end{table}
