# Supplementary material for: Video Instance Matting
Source: arXiv:2311.04212 source file (2023-11-08)
Supplement: Supplementary file 2 [file mask_perturbation.tex]

%MSG-VIM

%%%%%%%%%%%%%%%%%%%%%%%%%%%%%%%%

% 0% 
% MSE
% RQ: 0.9935
%TQ: 1.0
%MQ: 0.9857
%VMQ: 0.9793 

% MAD
% RQ: 0.9935
% TQ: 1.0
% MQ: 0.7859
% VMQ: 0.7808

% dtssd
%RQ: 0.9935
%TQ: 1.0
%MQ: 0.7913
%VMQ: 0.7862

%%%%%%%%%%%%%%%%%%%%%%%%%%%%%%%%

% 25% S&P noise  
% MSE
%RQ: 0.9828
%TQ: 1.0
%MQ: 0.9255
% VMQ: 0.9096

% MAD
%RQ: 0.9828
%TQ: 1.0
%MQ: 0.5586
%VMQ: 0.549

% dtssd
% RQ: 0.9828
% TQ: 1.0
% MQ: 0.4813
% VMQ: 0.4731

%%%%%%%%%%%%%%%%%%%%%%%%%%%%%%%%

% 50% S&P noise  
% MSE
%RQ: 0.9516
%TQ: 1.0
%MQ: 0.7646
%VMQ: 0.7276

% MAD
%RQ: 0.9516
%TQ: 1.0
%MQ: 0.1423
%VMQ: 0.1354

% dtssd
% RQ: 0.9516
% TQ: 1.0
% MQ: 0.1201
% VMQ: 0.1143

%%%%%%%%%%%%%%%%%%%%%%%%%%%%%%%%

% 75% S&P noise
% MSE
%RQ: 0.9047
%TQ: 1.0
%MQ: 0.5524
%VMQ: 0.4997

%MAD
%RQ: 0.9047
%TQ: 1.0
%MQ: 0.0388
% VMQ: 0.0351

%dtssd 
%RQ: 0.9047
%TQ: 1.0
%MQ: 0.0419
%VMQ: 0.0379

%%%%%%%%%%%%%%%%%%%%%%%%%%%%%%%%

% 100% S&P noise
% MSE
%RQ: 0.1161
%TQ: 0.1912
%MQ: 0.0005
%VMQ: 0.0

%MAD
%RQ: 0.1161
%TQ: 0.1912
%MQ: 0.0
%VMQ: 0.0

%dtssd 
%RQ: 0.1161
%TQ: 0.1912
%MQ: 0.0076
%VMQ: 0.0002


%Base Model 

%%%%%%%%%%%%%%%%%%%%%%%%%%%%%%%%

% 0% 
% MSE
%RQ: 0.9925
%TQ: 1.0
%MQ: 0.973
%VMQ: 0.9656

% MAD
%RQ: 0.9925
%TQ: 1.0
%MQ: 0.7813
%VMQ: 0.7754


% dtssd
%RQ: 0.9925
%TQ: 1.0
%MQ: 0.7864
%VMQ: 0.7805

%%%%%%%%%%%%%%%%%%%%%%%%%%%%%%%%

% 25% 
% MSE
%RQ: 0.8572
%TQ: 1.0
%MQ: 0.4459
%VMQ: 0.3823

% MAD
%RQ: 0.8572
%TQ: 1.0
%MQ: 0.0614
%VMQ: 0.0526

% dtssd
%RQ: 0.8572
%TQ: 1.0
%MQ: 0.0241
%VMQ: 0.0207

%%%%%%%%%%%%%%%%%%%%%%%%%%%%%%%%

% 50% 
% MSE
%RQ: 0.0026
%TQ: 0.02
%MQ: 0.0025
%VMQ: 0.0


% MAD
%RQ: 0.0026
%TQ: 0.02
%MQ: 0.0002
%VMQ: 0.0

% dtssd
%RQ: 0.0026
%TQ: 0.02
%MQ: 0.0004
%VMQ: 0.0

%%%%%%%%%%%%%%%%%%%%%%%%%%%%%%%%

% 75% 
% MSE
%
%RQ: 0.0
%TQ: 0.0
%MQ: 0.0
%VMQ: 0.0

% MAD
%RQ: 0.0
%TQ: 0.0
%MQ: 0.0
%VMQ: 0.0

% dtssd
%
%RQ: 0.0
%TQ: 0.0
%MQ: 0.0
%VMQ: 0.0


%%%%%%%%%%%%%%%%%%%%%%%%%%%%%%%%

% 100% 
% MSE
%RQ: 0.0
%TQ: 0.0
%MQ: 0.0
%VMQ: 0.0

% MAD
%RQ: 0.0
%TQ: 0.0
%MQ: 0.0
%VMQ: 0.0

% dtssd
%RQ: 0.0
%TQ: 0.0
%MQ: 0.0
%VMQ: 0.0



%%%%%%%%%%%%%%%%%%%%%%%%%%%%%%%%


% 25% 90.99 98.27 78.12 69.85
                % 58.91 52.68
                % 45.23 40.45
                
% 50% 90.74 98.21 77.32 68.91 
                 % 58.22 51.89
                % 44.28 39.46
                
% 75% 90.43 98.13 76.14 67.57
                % 57.28 50.83
                % 42.96 38.12

% 100% 90.35 98.07 75.99 67.33
                % 56.96 50.47
                % 42.22 37.41
