# Supplementary material for: Video Instance Matting
Source: arXiv:2311.04212 source file (2023-11-08)
Supplement: Supplementary file 3 [file speed.tex]

\begin{table}[tb]
\centering
\begin{tabular}{c|cc}
 Model  & Input Resolution  &  FPS   \\ \hline %&dtSSD$\downarrow$ \\ \hline
MSG-VIM  &$512 \times 288$ & 13.81 \\ 
MSG-VIM  &$1024 \times 576$ & 3.23 \\ 
MSG-VIM  &$1920 \times 1080$ &0.54 \\ 

\end{tabular}
\caption{Inference Speed of the MSG-VIM. We test the inference speed on a single A6000 GPU.}
\label{tab:speed}
\end{table}
